# Supplementary material for: Sequential vs. Integrated Algorithm Selection and Configuration: A Case Study for the Modular CMA-ES
Source: arXiv:1912.05899 source file (2020-01-06)
Supplement: Supplementary file 1 [file appendix.tex]

\appendix
\section{Impact of instance variation}
All experiments performed in this thesis have been aggregated over 5 instances of the selected benchmark function. However, it has previously been shown~\cite{BelkhirDSS17} that the optimal hyperparameter values might differ per instance. In this section, the data generated during the experiment described in Section~\ref{sec:baseline2} is analyzed to get an insight into the differences between the instances of the bbob-functions used. Figure~\ref{fig:ht_per_inst} shows the distributions of hitting times for each instance of each function. This shows us that some functions have very significant differences between their instances. The most obvious example is F12, for which the differences in hitting times are very significant. This matches previous observations from Section~\ref{sec:variance}, specifically Figure~\ref{fig:violins_F12}, in which we observed the clear multi-modality of the hitting times. \bigskip

\begin{figure}
    \centering
    \includegraphics[width=\textwidth, trim={50 60 30 80},clip]{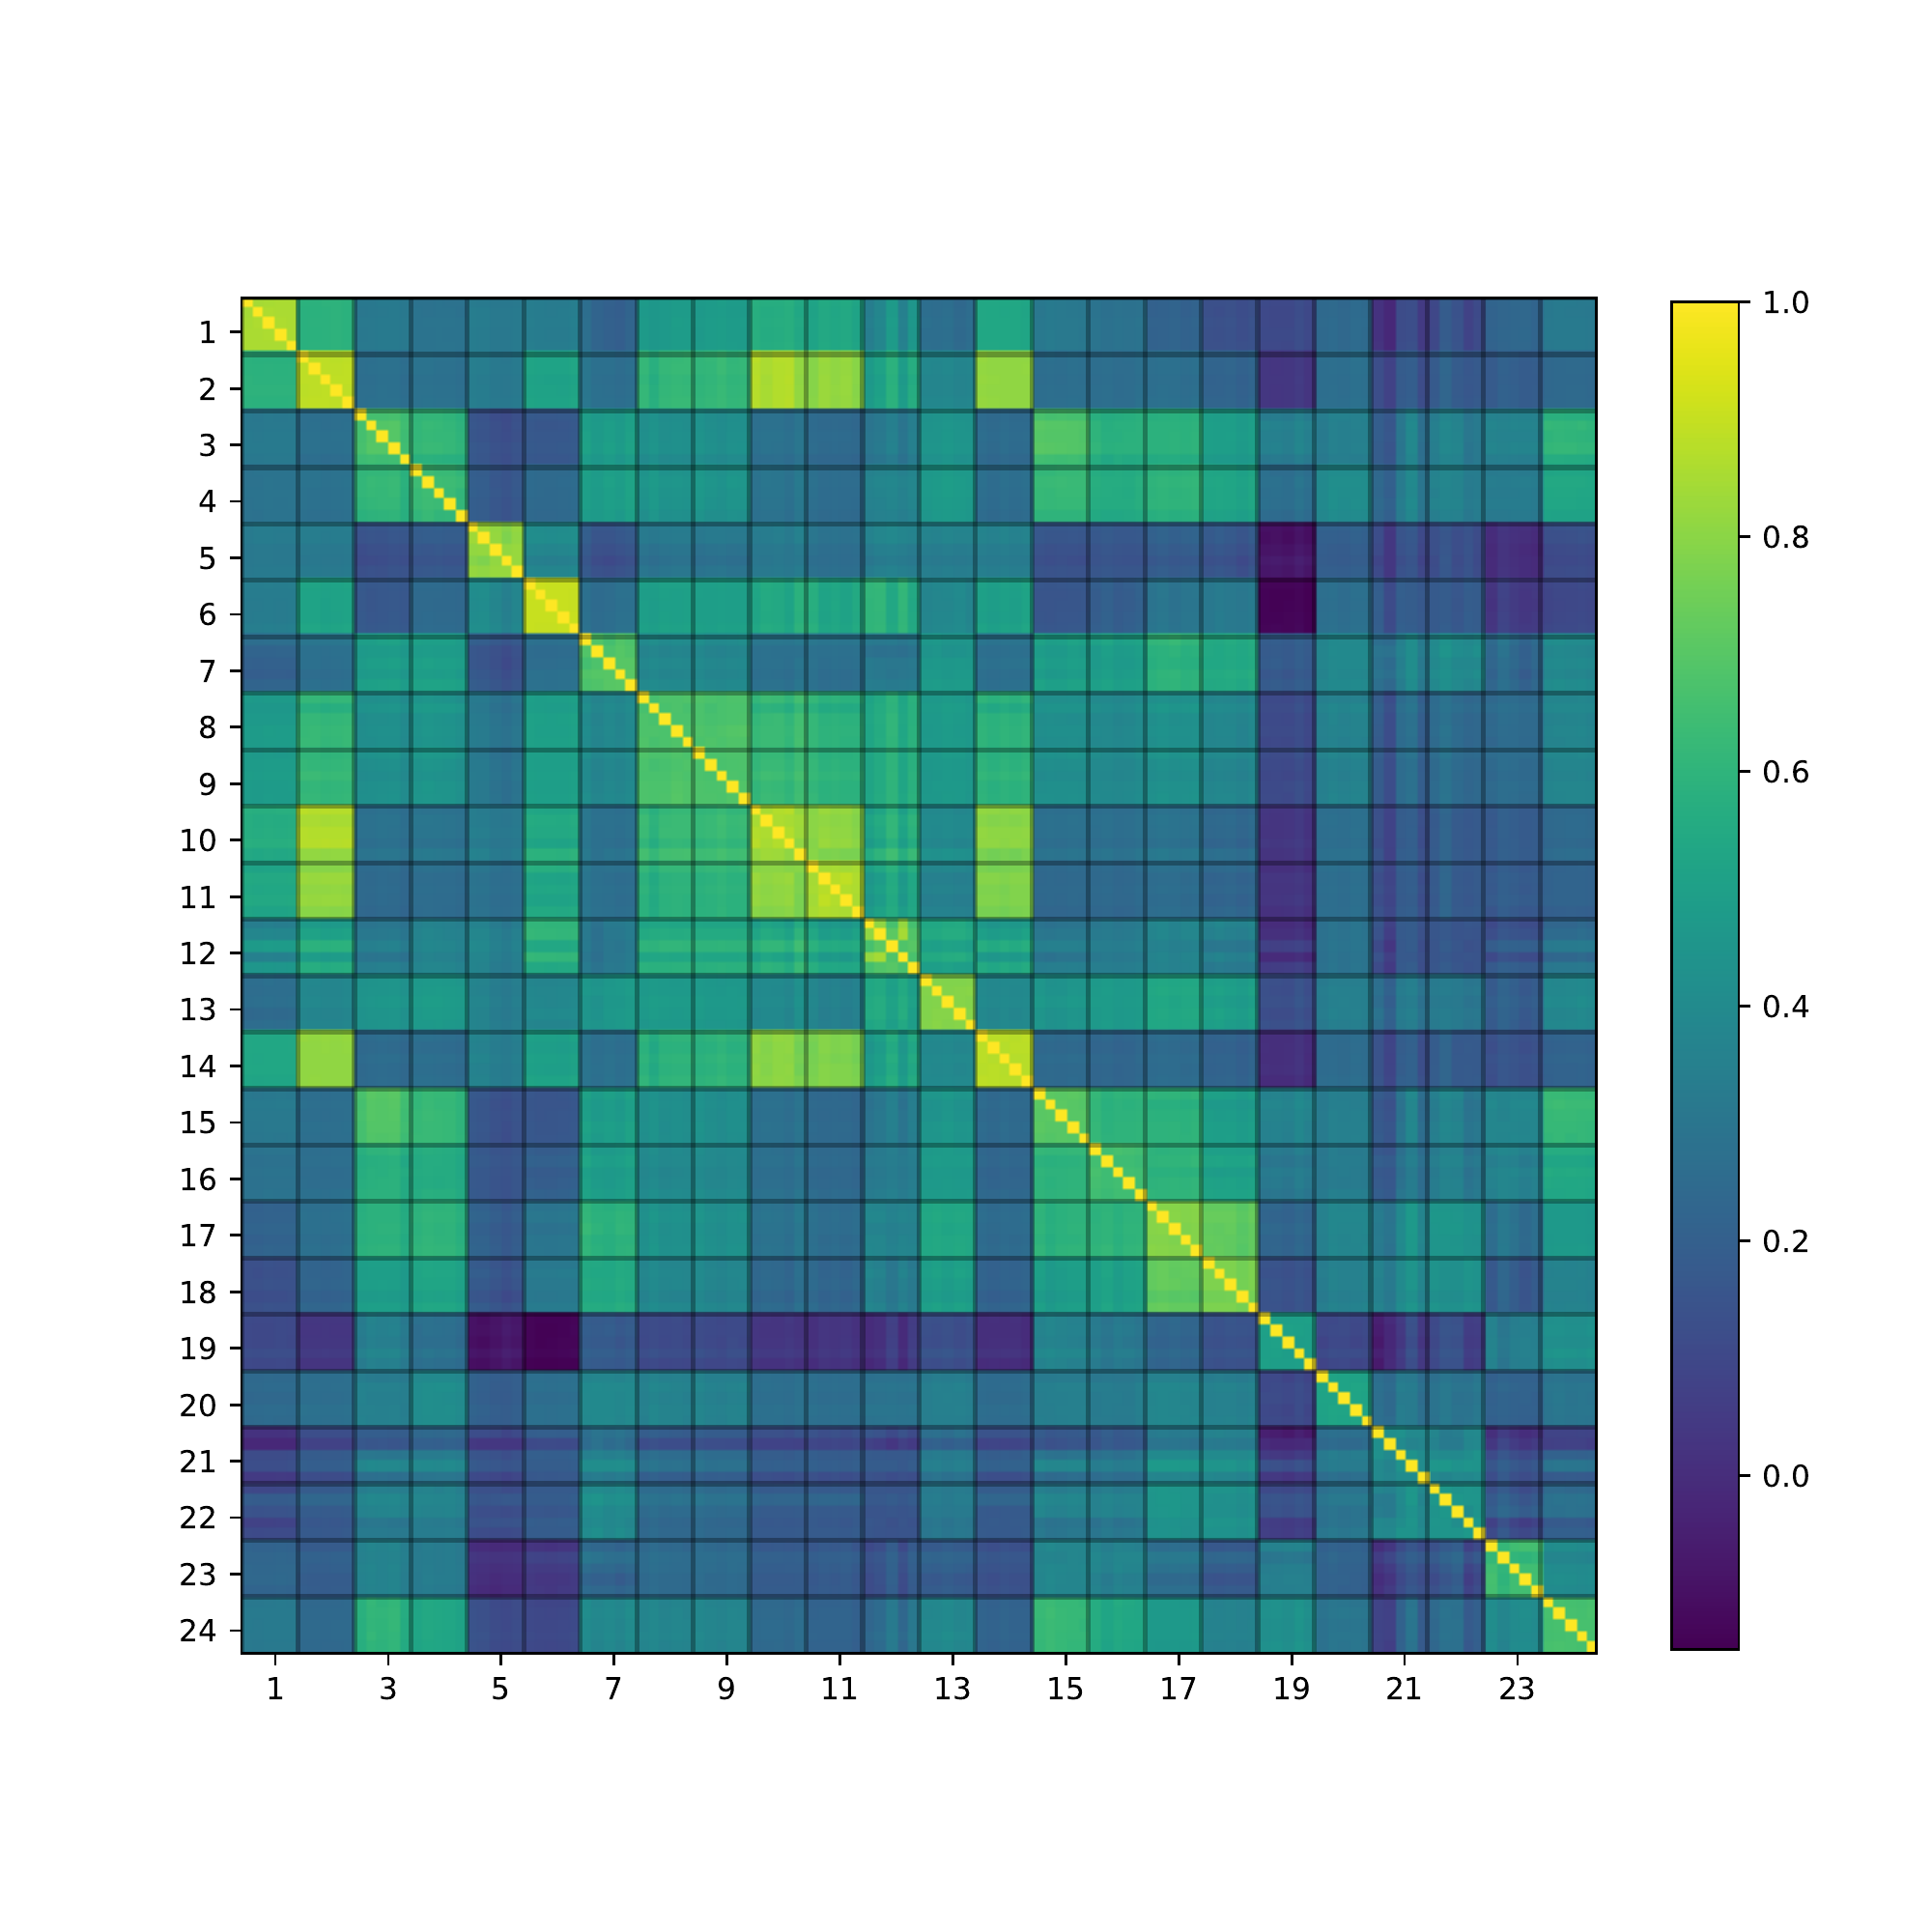}
    \caption{Kendall correlation of rankings of all configuration between instances of all benchmark functions. Rankings based on ERT from 5 runs per instance.}\vspace{-25pt}
    \label{fig:kendall_corr_matrix}
\end{figure}

\begin{figure}
    \centering
    \includegraphics[width=\textwidth, trim={30 80 60 110},clip]{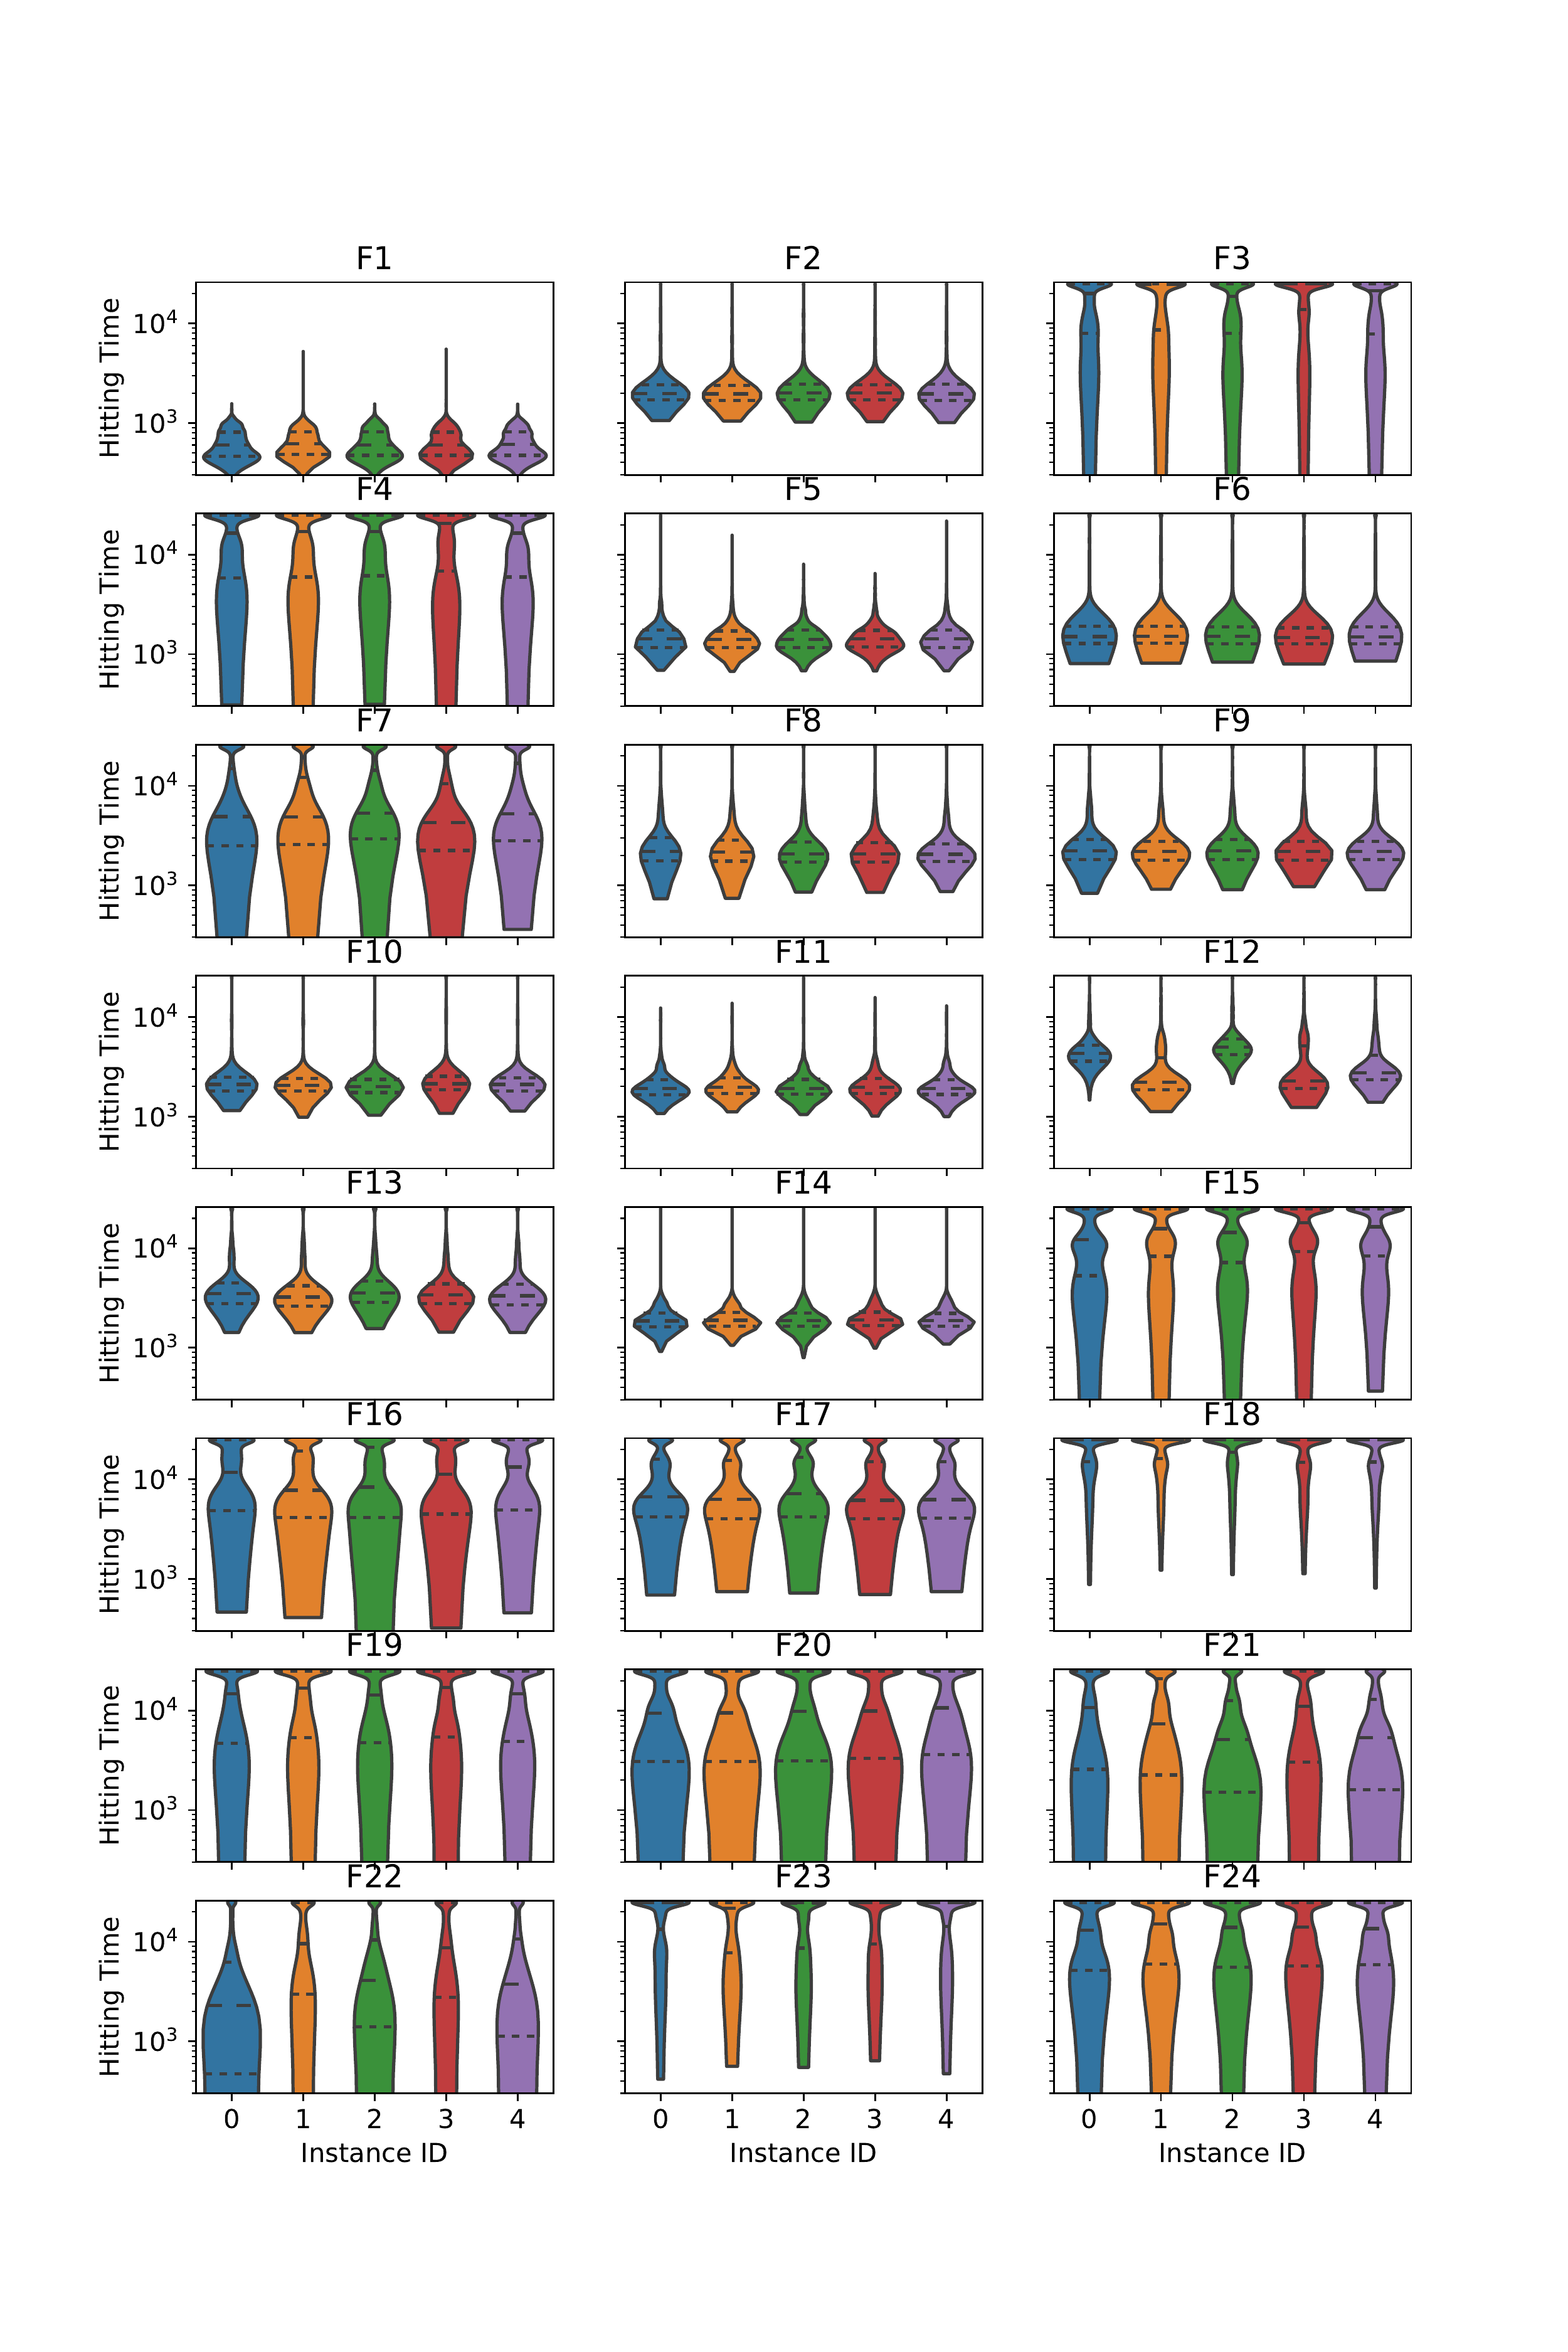}
    \caption{Distributions of hitting times per instance for all benchmark functions. All distributions are from 30 configurations (as described in Section~\ref{sec:baseline2}), each with tuned hyperparameters (using MIP-EGO) and run 50 times on each instance.}
    \label{fig:ht_per_inst}
\end{figure}

Another way to look at the differences between instances is to use the $5\times 5$ hitting time data, which is available for all configurations. Figure~\ref{fig:kendall_corr_matrix} shows the Kendall correlations between these rankings across 5 instances of all benchmark function. This seems to confirm the findings from Figure~\ref{fig:ht_per_inst}, in that for most functions the differences between their instances is quite small. For F12, there is also a clear distinction between some of the instances, which matches our previous observations.\bigskip

\newpage

\section{Configuration Switching}\label{sec:switching}
Previous work on modEA has introduced the concept of configuration switching~\cite{van_rijn_ppns_2018_adpative}. This is motivated by the fact that different configuration have different convergence behaviour. These differences might be exploited by starting with a configuration $c_1$ which reaches a certain target $\sigma$ with the fewest number of functions evaluations. We refer to this target $\sigma$ as the splitpoint, as once this target is hit, a switch is made to a different configuration $C_2$. This principle is visualized in Figure~\ref{fig:switch_example}.\bigskip

% A single-switch configuration is defined as a triple $(C_1,C_2,\sigma)$, where $C_1$ indicates the configuration used at the start of the optimization, $C_2$ the configuration to which is switched and $\sigma$ the target precision at which to switch, called the splitpoint. The motivation behind this kind of switch is illustrated in Figure~\ref{fig:switch_example}. \bigskip

In~\cite{research_project}, this configuration switching was implemented. Based on the results from this paper, we noticed that variance plays a big role in the performance of switching configurations. To mitigate this, a two-stage approach was developed to determine which switching configurations to run. This approach first gathers a collection of `interesting' configurations: the top 50 best static ones and the configurations used in the top 50 theoretically best switching ones (determined by complete enumeration). Then these configurations were run 250 times to get some more robust data on which to base the final selection of switching configurations. \bigskip

\begin{figure}[ht]
    \centering
    \includegraphics[width=\textwidth, trim={15 0 70 30},clip]{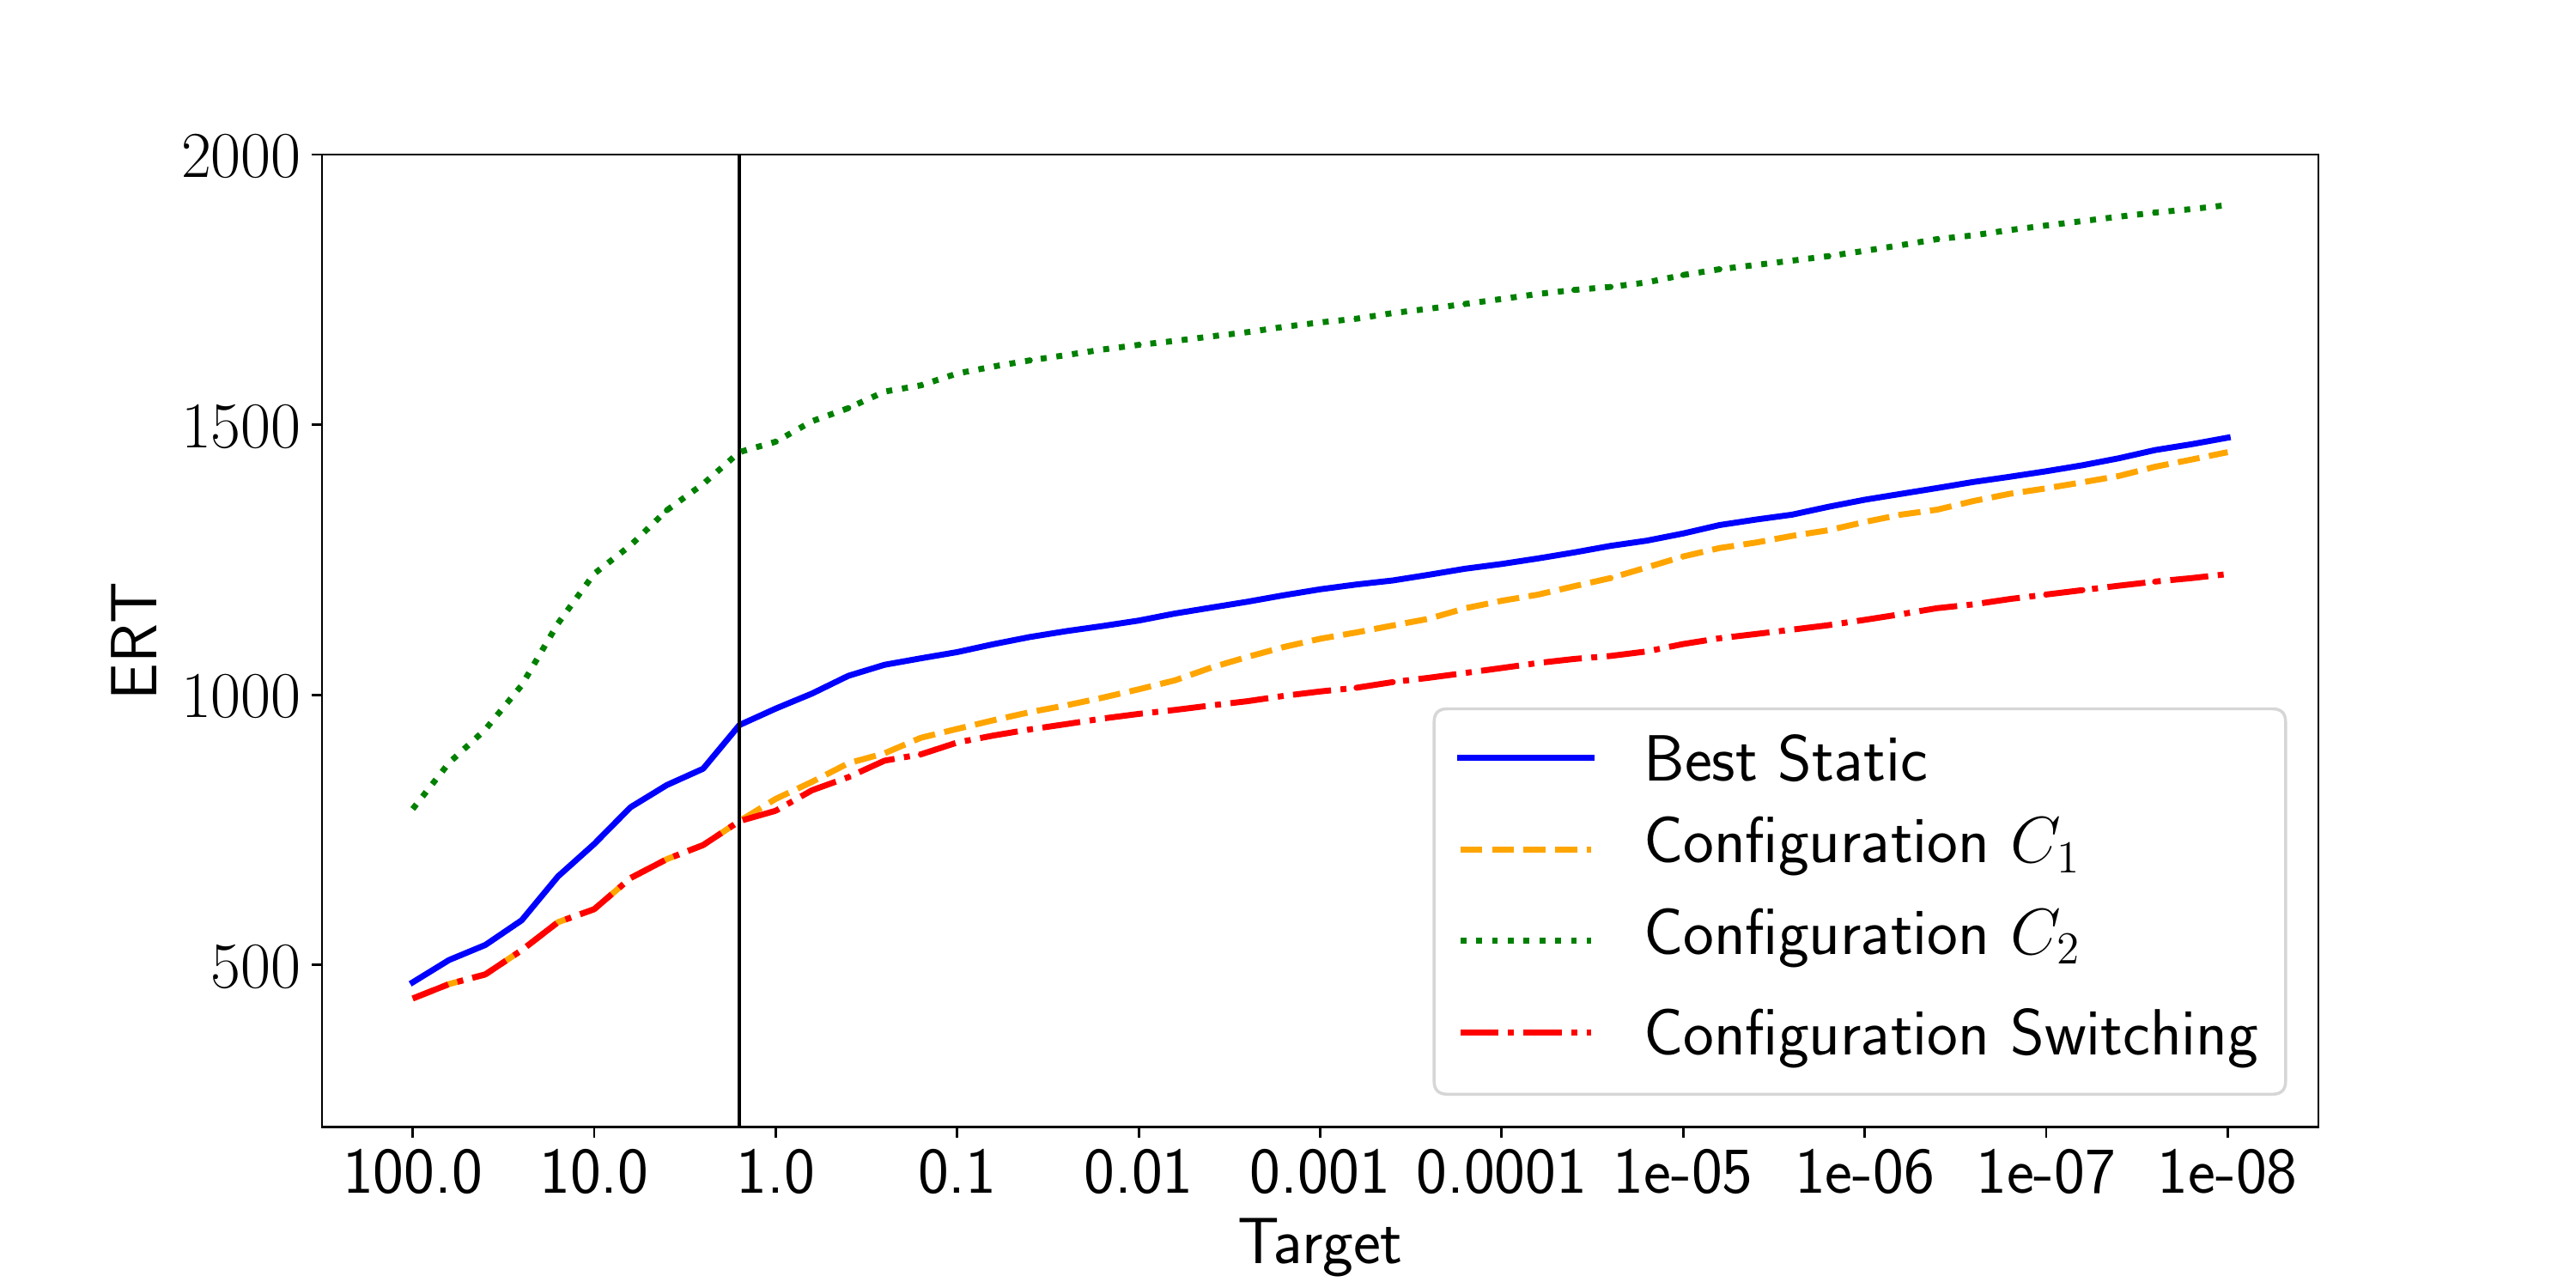}
    \caption{Example of how a configuration switch could theoretically outperform the best static configuration. It follows the convergence path of $C_1$ until the splitpoint $\sigma$, after which it follows the exact convergence behaviour of $C_2$, thus reaching the final target with less evaluations than the best static configuration.}
    \label{fig:switch_example}
\end{figure}

% We found that using this two-stage approach is promising for a subset of the 24 functions we tested on. However, especially for the more multimodal functions, it failed to find stable switching configurations. One of the reasons for this behaviour was that these functions benefit a lot from the (B)IPOP module, which was not used in the switching configurations. To remedy this and determine the best switching configurations with (B)IPOP enabled would require us to again rerun the two-stage approach and gather data from 250 runs for anywhere between 50 and 150 configurations. This is quite computationally inefficient, and not easily extendable, especially when the raw (25 run) data is not already available. Any new module added to the modEA framework would require gathering data for at least an additional $4,\hspace{-1pt}608$  configurations, which in practice requires months of CPU-time.\bigskip

\newpage

\section{Impact of budget on performance of irace}\label{app:irace}
In this thesis, the execution of the integrated algorithm selection and configuration has been performed with a fixed budget, namely $25,\hspace{-1pt}000$ evaluations. However, this is a rather arbitrary limit, and similar results might be achieved with a much lower budget. To test this hypothesis, another experiment was performed: For several different budget values, 3 runs of irace were performed on F12. As always, the resulting (configuration, hyperparameters)-pairs from this experiment are then run 250 times to allow for a fair comparison. The hitting time distributions resulting from these runs are visualized in Figure~\ref{fig:budget_F12_irace}.\bigskip 

\begin{figure}[!hb]
    \centering
    \includegraphics[width=\textwidth, trim={25 5 70 50},clip]{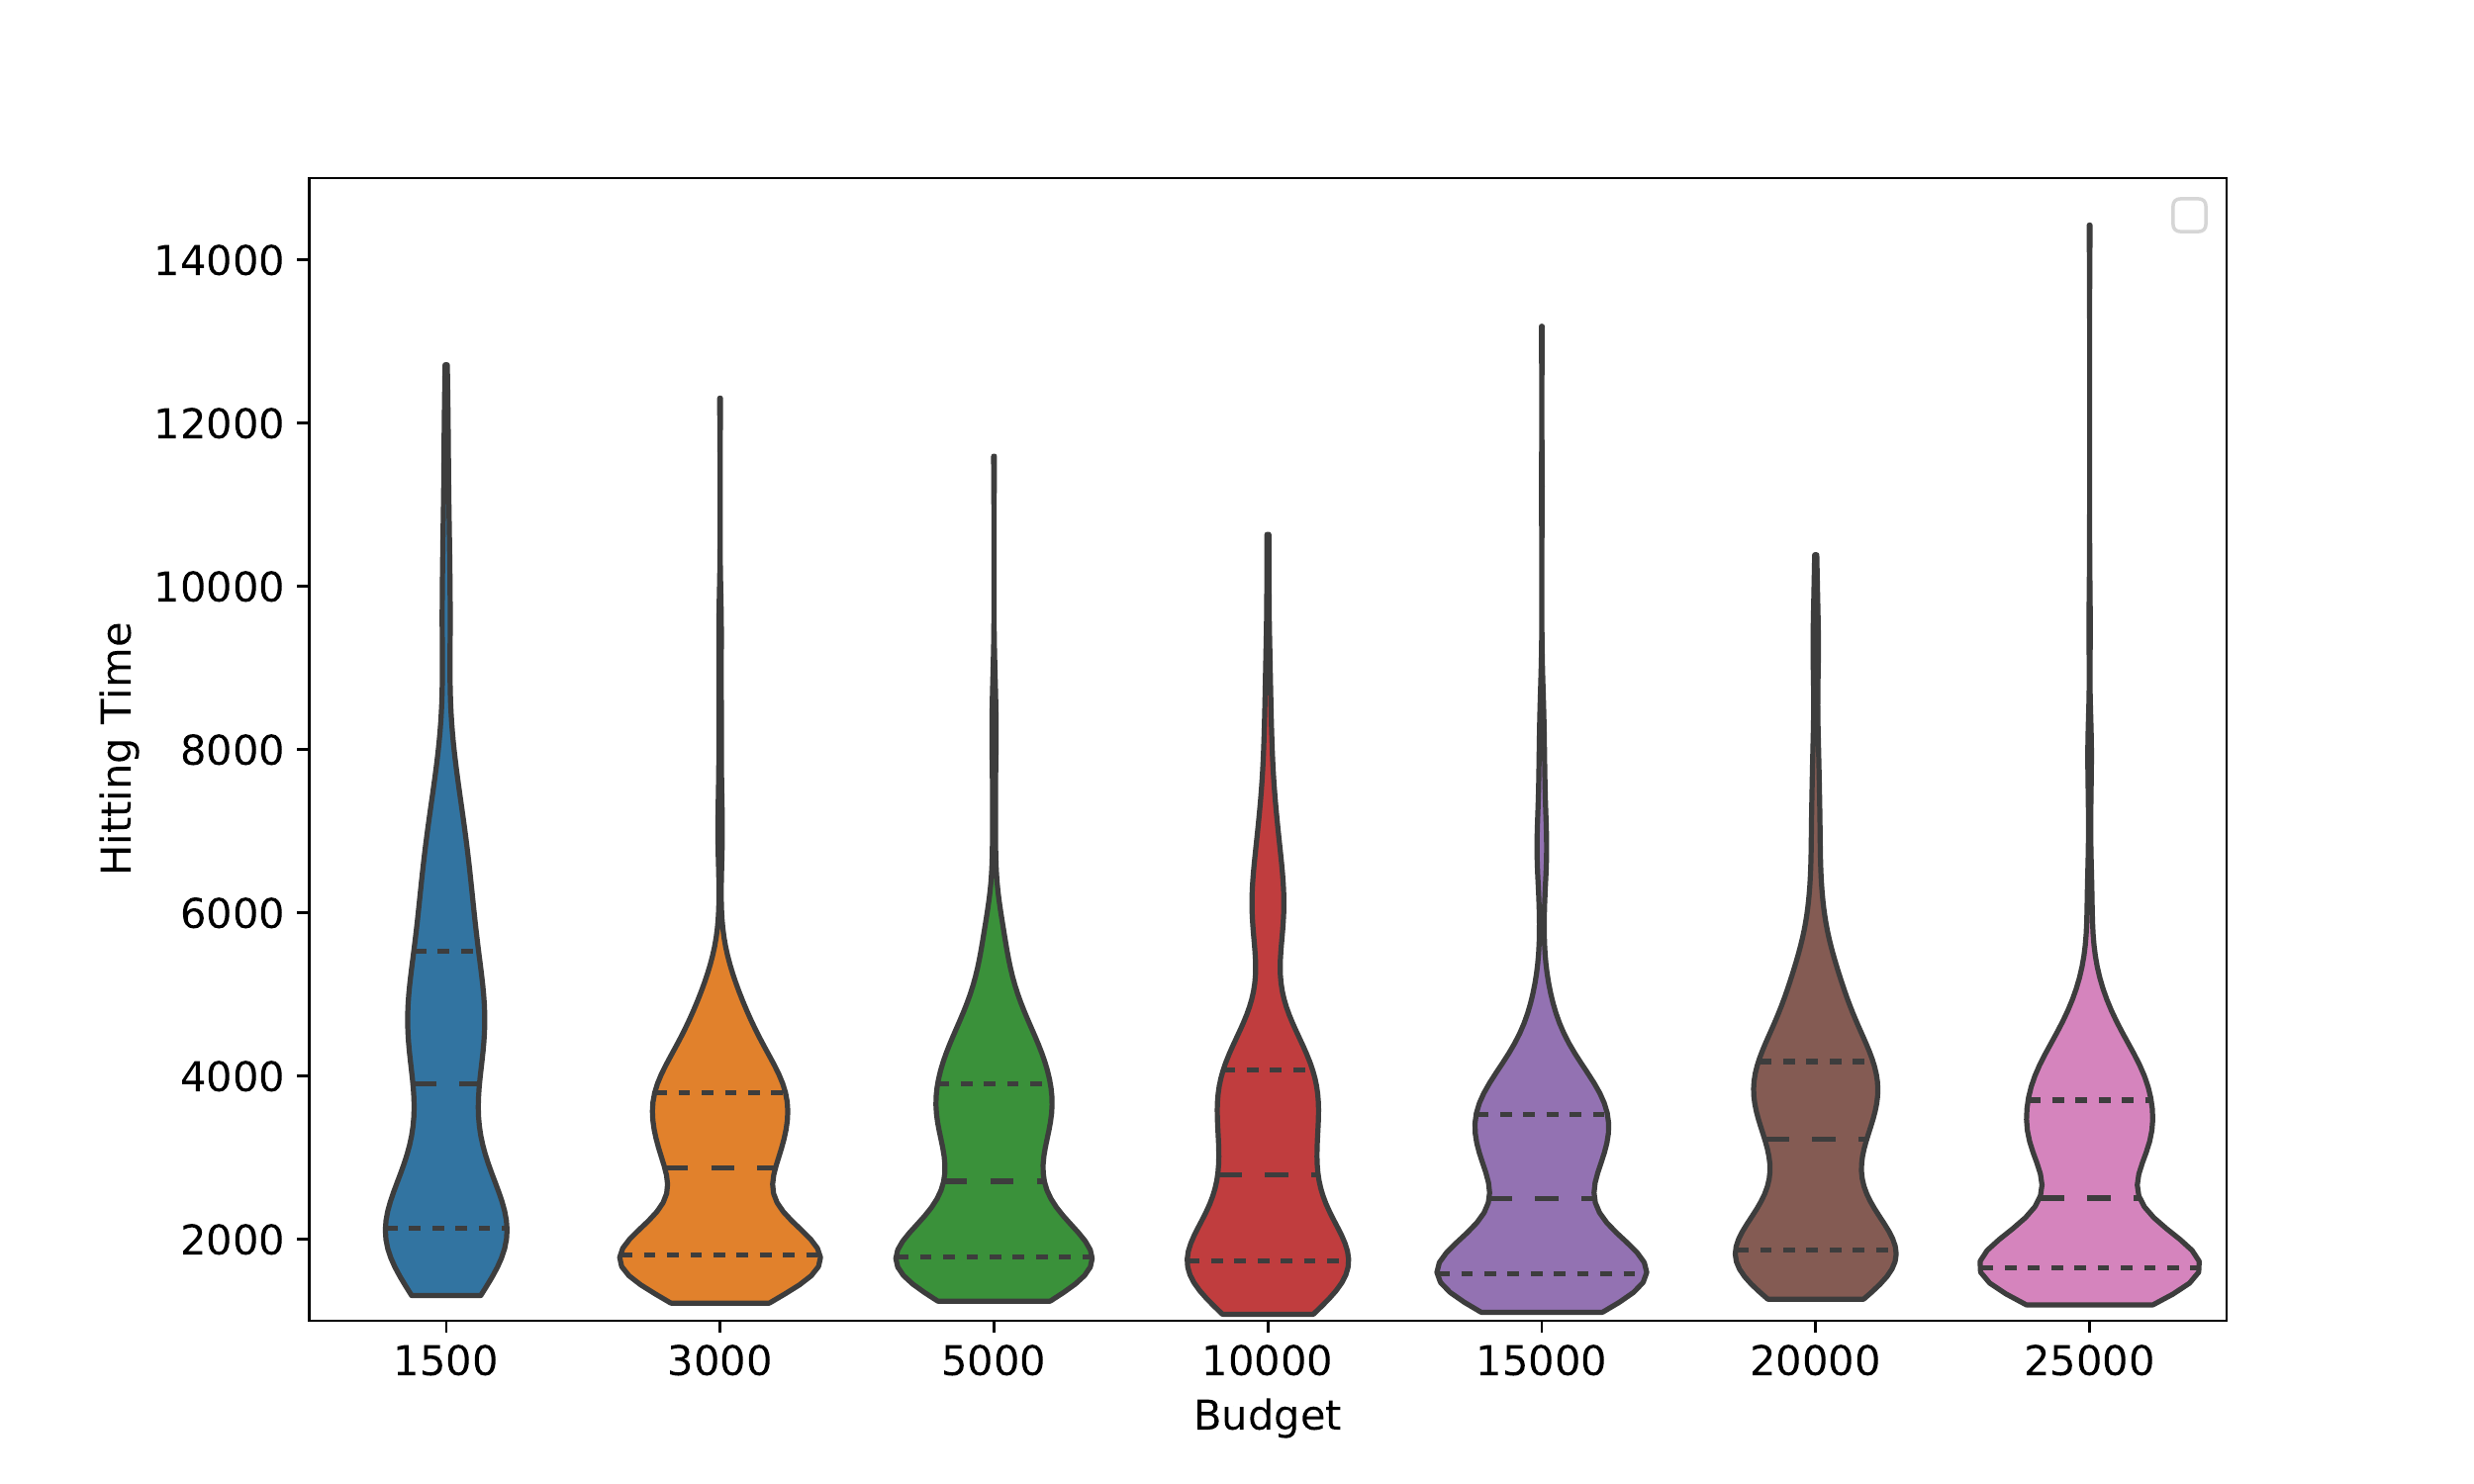}
    \caption{Hitting time distributions from (configuration, hyperparameters)-pairs as determined by irace using different budgets. Hitting times are from 3 runs of irace, for 250 runs each, for a total of 750 runs per budget-value.}
    \label{fig:budget_F12_irace}
\end{figure}

From Figure~\ref{fig:budget_F12_irace}, it can be seen that the differences in performance between different budget values are present, but not very large. For the lower budget values, the hitting times have a much higher variance, which might point to a larger prediction error, since a distribution with high variance might get picked over a better one with low variance when very few samples are selected. To verify this, we calculated the average prediction error for each budget value. These are visualized in Figure~\ref{fig:budget_F12_pred_errs}. While this shows clearly that 3 samples is too little to make any definitive statements, it seems like the prediction error is only slightly worse for the lowest budget values compared to the highest. \bigskip

\begin{figure}[!htbp]
    \centering
    \includegraphics[width=\textwidth, trim={25 5 70 50},clip]{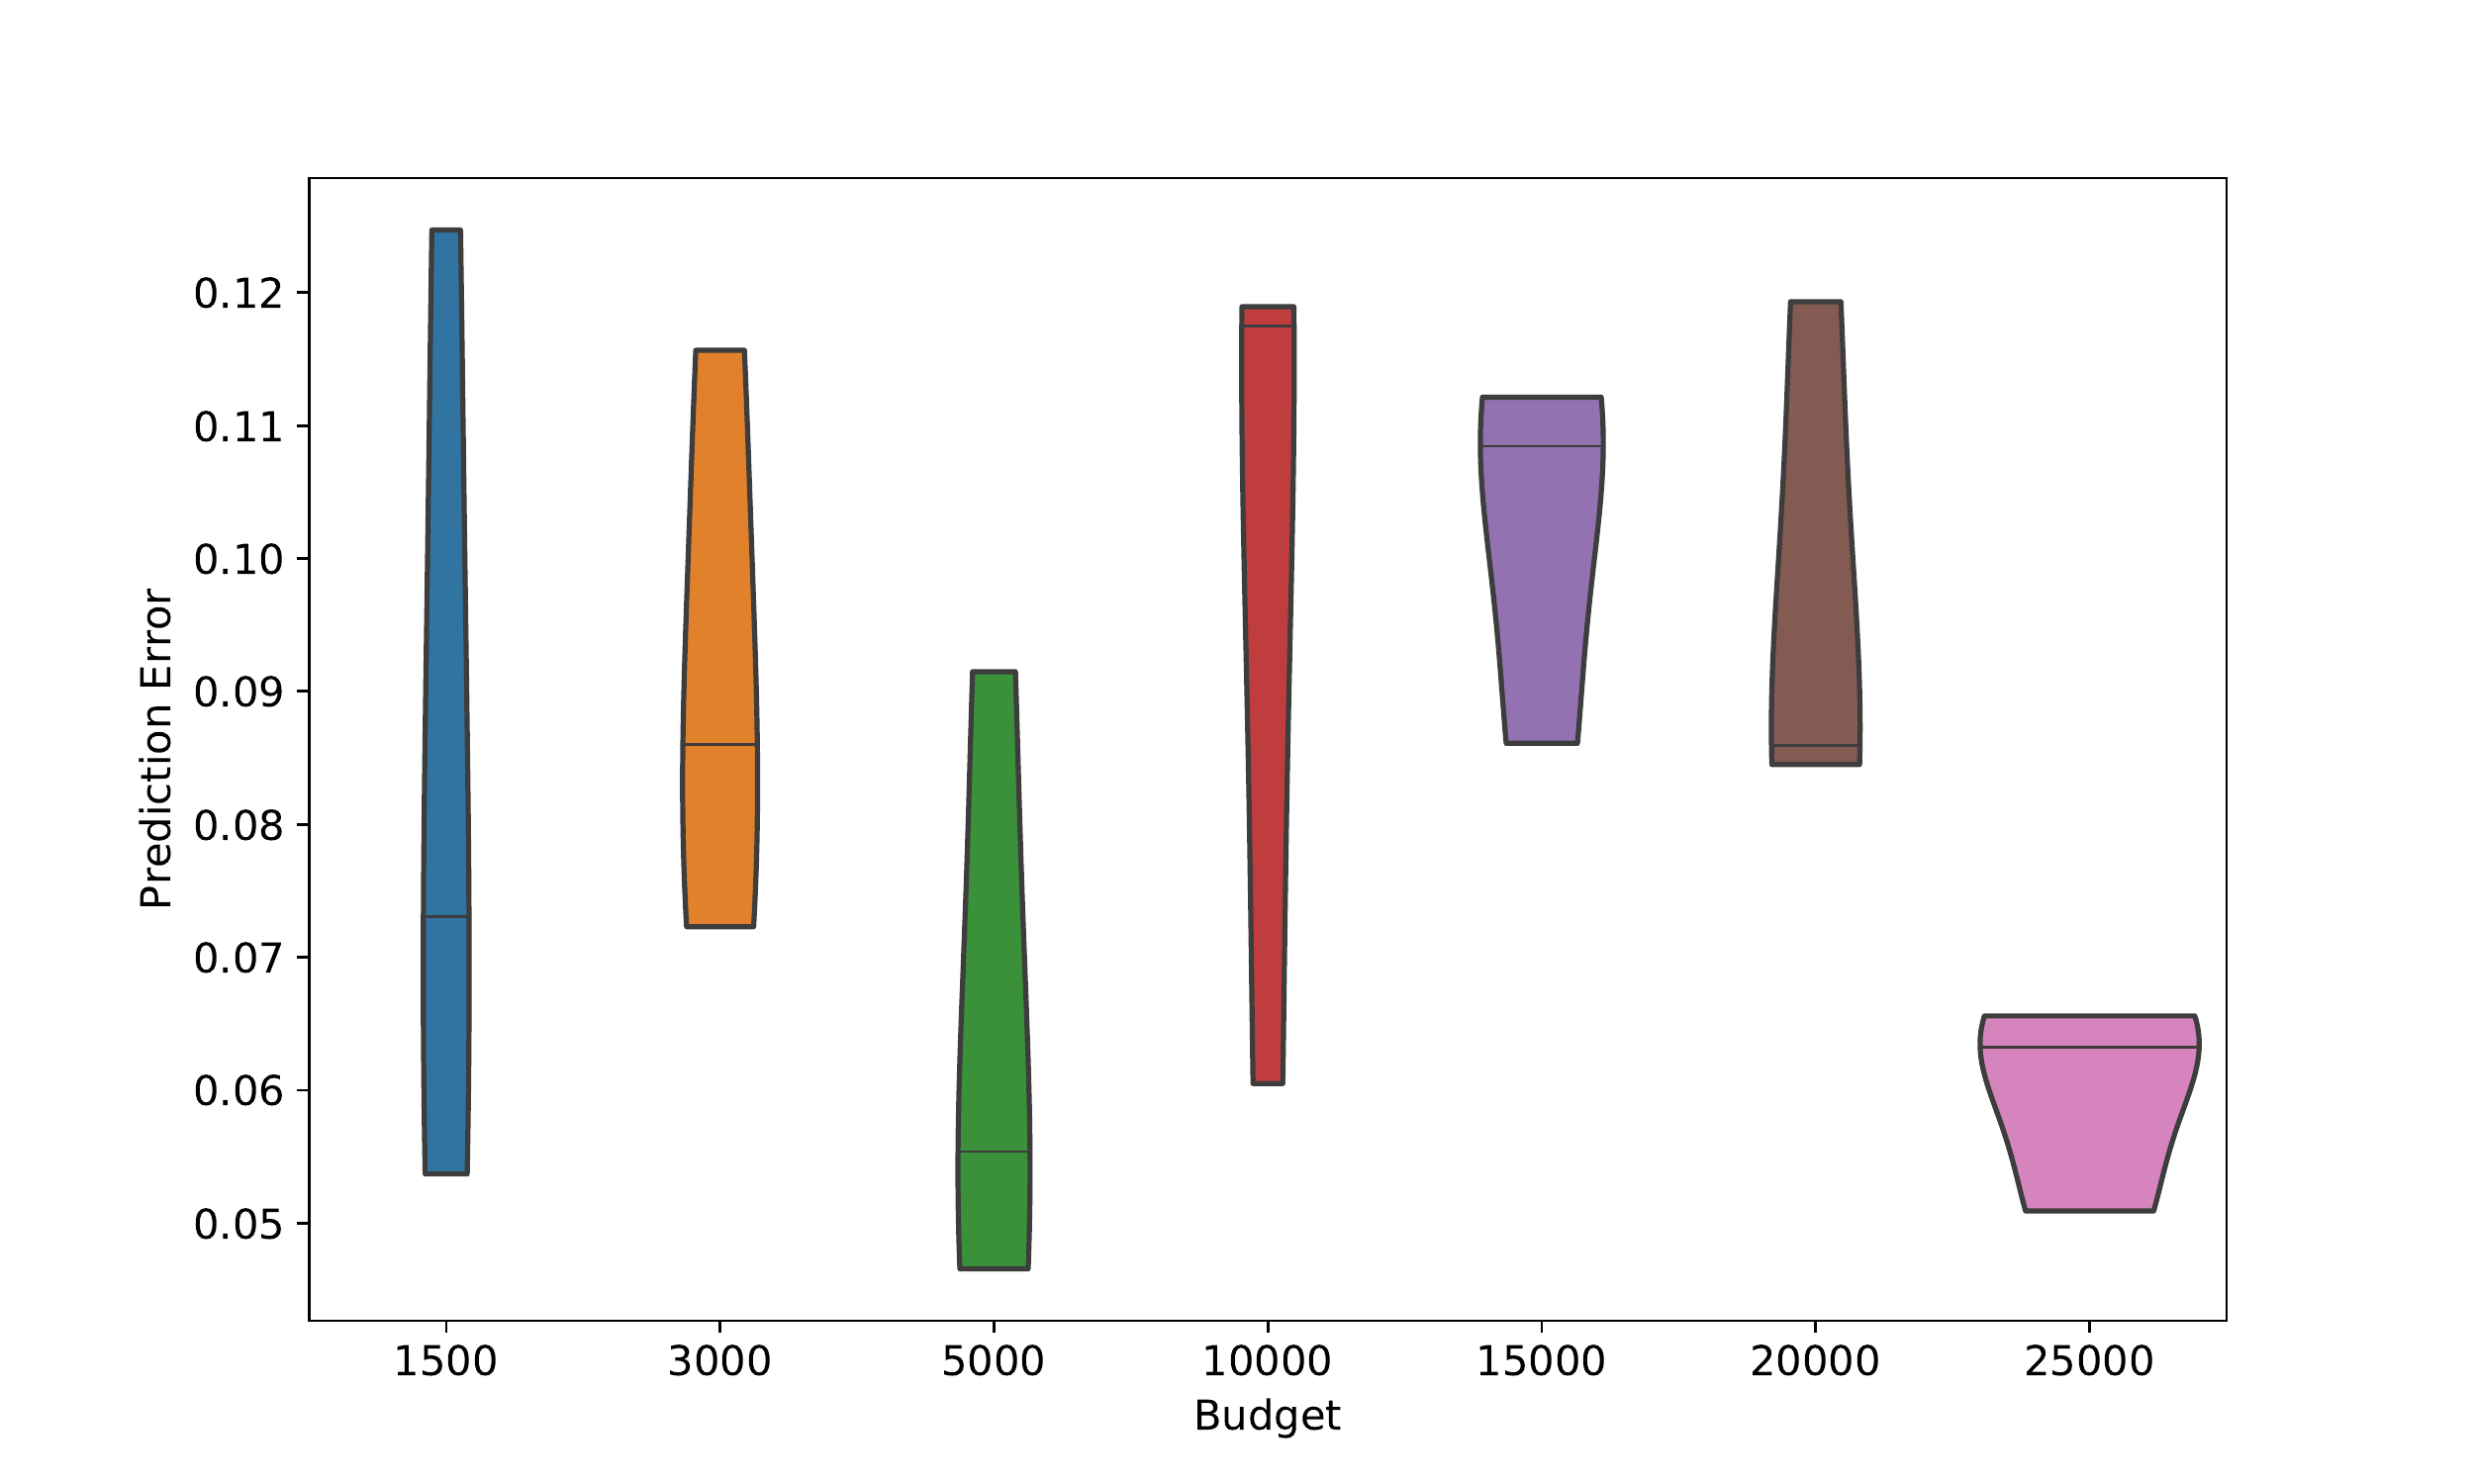}
    \caption{Distributions of prediction errors from (configuration, hyperparameters)-pairs as determined by irace using different budgets. Each is based on 3 runs of irace, comparing the ERT for 250 runs to the predicted ERT.}
    \label{fig:budget_F12_pred_errs}
\end{figure}

While the scope of this experiment is too small to draw any real conclusions, it seems to indicate that a smaller budget might work similarly well to the $25,\hspace{-1pt}000$ which was used in this thesis. A more robust search into the optimal budget value might be done in future work, but is outside of the scope of this project, as this only aims to prove the viability of the integrated algorithm selection and configuration method, which is still shown with a budget of $25,\hspace{-1pt}000$.

\newpage

\section{Parsing Configuration IDs}\label{app:mod_conf}
Throughout this thesis, we refer to configurations within the modEA framework by their configuration ID. This number uniquely represents the configuration in terms of its module configuration. To convert the module activations vector into their configuration ID, we can use the following algorithm:
$$\text{ConfID}(\Vec{m}) = \begin{bmatrix}2304& 1152& 576& 288& 144& 72& 36& 18& 9& 3& 1\end{bmatrix} \cdot \begin{bmatrix}m_1 \\ \vdots \\ m_{11}\end{bmatrix}$$
Where $m_x$ indicates the value of module number $x$, as in Table~\ref{tab:es-opt}. To convert from configuration ID to module activations, the inverse function is used.

\begin{sidewaystable}[!hbp]
    \centering
    \small
\begin{tabular}{
 @{}p{0.03\linewidth}
    p{0.05\linewidth}
    p{0.05\linewidth}
    >{\raggedleft\arraybackslash}p{0.05\linewidth}
    p{0.05\linewidth}
    >{\raggedleft\arraybackslash}p{0.05\linewidth}
    >{\raggedleft\arraybackslash}p{0.05\linewidth}
    p{0.05\linewidth}
    >{\raggedleft\arraybackslash}p{0.05\linewidth}
    p{0.05\linewidth}
    >{\raggedleft\arraybackslash}p{0.05\linewidth}
    p{0.05\linewidth}
    >{\raggedleft\arraybackslash}p{0.05\linewidth}
    p{0.05\linewidth}
    >{\raggedleft\arraybackslash}p{0.05\linewidth}@{}
    }
\toprule
FID &   Target &  Common Conf & Common ERT &  Static Conf (25) & Static ERT (25) & Static Tuned ERT &  Static Conf (250) & Static ERT (250) &  Seq. Conf & Seq. ERT &  MIP-EGO Conf & MIP-EGO ERT &  Irace Conf & Irace ERT \\
\midrule
1        &  10e-8.0 &         1152 &        521 &               921 &             447 &              456 &               3227 &              445 &             3229 &            \textbf{392} &           903 &         487 &        4598 &       436 \\
2        &  10e-8.0 &            0 &      1,781 &              3714 &           2,042 &            1,921 &               1281 &            1,711 &             4585 &          1,573 &          1264 &       \textbf{1,438} &         867 &     1,501 \\
3        &   10e0.4 &            2 &     16,655 &               869 &          12,828 &           12,604 &                872 &           11,896 &              149 &         \textbf{11,688} &           617 &      19,158 &        3173 &    12,221 \\
4        &   10e0.8 &         2306 &     12,869 &               884 &          11,933 &           12,896 &                599 &           11,866 &              896 &         12,747 &          1028 &      14,043 &         884 &    \textbf{11,767} \\
5        &  10e-8.0 &          594 &      1,254 &              1311 &           1,607 &            1,540 &               1010 &            1,539 &             3190 &          \textbf{1,115} &          1034 &       1,148 &        1029 &     1,128 \\
6        &  10e-8.0 &         3457 &      1,363 &              2166 &           1,354 &            1,120 &               2039 &            1,271 &             2165 &          \textbf{1,102} &          2176 &       1,224 &        1902 &     1,156 \\
7        &  10e-8.0 &            2 &      3,936 &              3208 &           4,439 &            3,525 &               1436 &            3,468 &               40 &          3,071 &          1570 &       3,577 &        1274 &     \textbf{2,527} \\
8        &  10e-8.0 &         3458 &      2,710 &              1016 &           1,985 &            1,884 &                866 &            1,891 &              864 &          1,872 &           869 &      \textbf{1,774} &        3176 &     1,790 \\
9        &  10e-8.0 &         2306 &      2,704 &              1015 &           2,045 &            2,068 &                870 &            1,931 &              869 &          \textbf{1,695} &           869 &       1,983 &        3176 &     1,742 \\
10       &  10e-8.0 &            0 &      1,898 &              3572 &           2,161 &            2,043 &               1309 &            1,882 &             1008 &          1,615 &           867 &       \textbf{1,465} &         885 &     1,493 \\
11       &  10e-8.0 &            1 &      1,822 &              2706 &           1,872 &            1,872 &               3281 &            1,467 &             3281 &          1,472 &          3281 &       1,522 &        3208 &     \textbf{1,443} \\
12       &  10e-8.0 &          594 &      3,930 &              2019 &           3,568 &            3,422 &                864 &            3,096 &              864 &          2,825 &          3172 &       \textbf{2,655} &        1030 &     3,037 \\
13       &  10e-8.0 &            0 &      2,847 &              1166 &           3,241 &            3,100 &               1166 &            3,350 &             3188 &          2,740 &          2596 &       \textbf{2,517} &        2308 &     2,544 \\
14       &  10e-8.0 &            0 &      1,714 &              1267 &           1,912 &            1,873 &               1418 &            1,625 &             1418 &          1,538 &          3317 &       1,432 &           3 &     \textbf{1,372} \\
15       &   10e0.4 &            2 &     13,975 &               865 &          15,351 &           15,043 &                872 &            8,145 &             1013 &          8,629 &          3317 &       9,515 &        1013 &     \textbf{7,854} \\
16       &  10e-2.0 &            2 &      9,784 &              3187 &          12,035 &           10,614 &                890 &            5,437 &              887 &          \textbf{5,245} &           896 &       5,864 &         890 &     5,579 \\
17       &  10e-4.4 &         2305 &      7,257 &               869 &           2,889 &            2,859 &                872 &            2,658 &              869 &          2,859 &           869 &       3,418 &         866 &     \textbf{2,840} \\
18       &  10e-4.0 &            1 &     16,234 &               865 &          18,383 &           19,915 &               1664 &           15,968 &             1664 &         11,149 &          4118 &       \textbf{5,312} &        2099 &     5,740 \\
19       &  10e-0.6 &            2 &     11,261 &               586 &          17,810 &           10,295 &                590 &           11,886 &              590 &          \textbf{7,718} &          3173 &       8,113 &        3181 &    11,357 \\
20       &   10e0.2 &            2 &      9,723 &              4379 &          11,439 &           11,174 &               1988 &            9,313 &             1988 &          \textbf{8,505} &           440 &      10,307 &        3860 &     9,671 \\
21       &  10e-0.6 &         3458 &      8,489 &              4343 &          11,149 &            9,713 &               1283 &            8,406 &             2900 &          2,939 &          2614 &       \textbf{2,831} &        2470 &     2,931 \\
22       &   10e0.0 &         3458 &      4,473 &              1592 &           4,767 &            5,097 &               2039 &            4,957 &             3458 &          4,564 &          2610 &       \textbf{3,582} &        1337 &     6,699 \\
23       &  10e-0.8 &          594 &     15,472 &               872 &          17,549 &           13,916 &                866 &           16,566 &              866 &         13,912 &           869 &     \textbf{12,938} &        4145 &    25,812 \\
24       &   10e1.0 &            2 &     12,475 &              2882 &           8,272 &            7,071 &                881 &            6,117 &             3029 &          \textbf{5,893} &          1016 &       7,950 &         878 &     6,653 \\
\bottomrule
\end{tabular}
\caption{Comparison of all methods discussed in this thesis. For each function, the used target value is selected in accordance with Table 3 from~\cite{research_project}. All columns with `conf' represent configuration numbers. The common configurations are taken from Table~\ref{tab:common}. Static (25) refers to the best configuration based on the 25 hitting times available for all configurations, while Static (250) refers to the best configuration after rerunning the set of configurations from Section~\ref{sec:baseline2} and selecting the one with the best ERT on 250 runs. Static tuned ERT is the same as the naive sequential approach, while Seq. refers to the sequential approach as described in Section~\ref{sec:baseline2}. All ERT data is based on hitting times for 50 runs on 5 instances. The lowest ERTs per function are bolded. }\label{tab:appendix_overview_table}
\end{sidewaystable}
